# Supplementary material for: Enhancing the Coherence of a Spin Qubit by Operating it as a Feedback Loop That Controls its Nuclear Spin Bath
Source: arXiv:1003.4031 ancillary file (2010-11-27)
Supplement: Supplementary file 1 [file supplement.pdf]

# Enhancing the Coherence of a Spin Qubit by Operating it as a Feedback Loop Controlling its Nuclear Spin Bath - Supplementary Information

Hendrik Bluhm,[1] Sandra Foletti,[1] Diana Mahalu,[2] Vladimir Umansky,[2] and Amir Yacoby[1]
[1]Department of Physics, Harvard University, Cambridge, MA 02138, USA
[2]Braun Center for Submicron Research, Department of Condensed Matter Physics, Weizmann Institute of Science, Rehovot 76100, Israel

This supplementary document provides additional information regarding the experimental procedures and pump rate measurements.

### Data acquisition

An improvement of our signal to noise ratio allowed us to increase the acquisition rate by a factor 30 compared to Ref. [1]. The $P_S$ vs. $\tau_S$ curves as shown in the inset to Fig. 2(a) were sampled at a rate of 32 data points per second, so that the whole curve can be acquired within 0.55 s. The actual sample rate of $\Delta B^z_{nuc}$ was reduced to about 1 Hz by the time required for data transfer and polarization between measurements, with the precise value depending on the polarization time.

For software feedback and measurements of the pump rate, we applied the pump pulses after every 10-20 measurements, each lasting 1/32 seconds. For the pulse feedback data shown in Figs. 3(b),(d), we pumped after each measurement of a single $\tau_S$, resulting in a total duration of the measurement-and-pump cycle of 100 ms. Slower repetition rates still work, but tend to result in larger fluctuations because of the longer time intervals of unstabilized fluctuations between pump cycles. Furthermore, the length of the pump intervals is limited by the requirement that $\Delta B^z_{nuc}$ does not leave the region of attraction of the desired fixed point before switching the pump pulse.

### Determination of pump times

In order to obtain a stable fixed point by combining $T_+$-pump and feedback pulses, we initially chose the pump times such that the $T_+$-pumping pulse alone reduces the gradient $\Delta B^z_{nuc}$ approximately at half the rate at which $S$-pumping increases it. Thus, the fixed point where the effects of the two pulses cancel should be at a singlet probability of 1/2, where the feedback gain $|\partial P_S/\partial \Delta B^z_{nuc}|$ is largest. We have verified that the effect of combining different pump pulses is qualitatively additive by comparing the pump rate of the $S$ and $T_+$ pulses individually to that of the combination.

We typically used a $\tau_{FB}$ between 15 and 30 ns. Larger $\tau_{FB}$ slightly improve $T_2^*$, but increase the frequency of occasional jumps between adjacent fixed points due to fluctuations. The frequency of such switching events can be minimized by fine tuning the ratio of $T_+$ and feedback pumping, and it is possible to return to the desired stable value of $\Delta B^z_{nuc}$ by temporarily using a different pump pulse or time.

### Pump rates

In order to obtain the pump rate data as plotted in Figs. 2(b) and (c), we run the $S$ or feedback pumping pulses until the gradient $\Delta B^z_{nuc}$ exceeds a predetermined threshold, at which point the acquisition software switches to the $T_+$-pumping cycle. When the value of the gradient falls below a second lower threshold, the software switches back to $S$ or feedback pumping. In the absence of fluctuations, the polarization effect of the feedback pulse would be expected to stagnate indefinitely at the plateaus visible in Fig. 2(c). Pumping indeed tends to stop for shorter $\tau_{FB}$, where the pump probability varies less rapidly with $\Delta B^z_{nuc}$. For $\tau_{FB} \gtrsim 15$ ns, fluctuations lead to a finite dwell time at those unstable fixed points.

The raw data obtained from repeating many of the above cycles is a series of curves of $P_S$ vs. $\tau_S$ as shown in the inset of Fig. 2(a). Obtaining the oscillation frequencies by fitting a sine curve to each of them results in time traces of $\Delta B^z_{nuc}$, part of which are shown in Figs. 2(b) and (c). Taking the difference between subsequent values yields a time trace of the pump rate, $\Delta B^z_{nuc}(t)/dt$, which is rather noisy because of the numerical differentiation. To average out this noise, we have binned this trace according to the corresponding values of $\Delta B^z_{nuc}$, and computed the mean $\Delta B^z_{nuc}(t)/dt$ for each bin, as shown in Fig. 2(d). The curves in Fig. 2(e) were obtained by applying the same binning procedure to the $P_S$ value for $\tau_S$ = 15 and 16 ns taken from each $\tau_S$ sweep.

The bare polarization rate, obtained at small $\Delta B^z_{nuc}$ where relaxation is weak, can reach values of up to 40 mT/s. The relaxation rate, which determines the slope of the pump curves in Fig. 2(d), depends on the pumping history, as expected for diffusive relaxation. The largest pump rates observed at $B_{ext} = 0.7$ T correspond to about one nuclear spin flip per 150 cycles. While our measurements of the rate of change of $\Delta B^z_{nuc}$ is sensitive to the difference between the flip probabilities in each dot, we found that the field gradient $\Delta B^z_{nuc}$ and the mean hyperfine field $B^z_{nuc}$ tend to be of the same order [1]. Thus,

the total spin flip probability should be similar to the measured differential value.

When sweeping through the $S$-$T_+$ transition, $\varepsilon$ is ramped by about 50 $\mu$eV in 50 ns, whereas the expected hyperfine coupling is $g^* \mu_B \delta B^z_{nuc} = 70$ neV. Setting $dJ/d\varepsilon$ to one, which becomes accurate for large fields with a Zeeman splitting much larger than the inter-dot tunnel coupling, the Landau-Zener formula would predict a flip probability of $1 - \exp(-2\pi(0.07\mu\text{eV})^2/(\hbar \cdot 1\mu\text{eV/ns})) \approx 0.05$. The magnetic field used in the experiments is comparable to rather than much larger than the tunnel coupling, which would increase the actual flip probability. On the other hand, the discreteness of the ramps with steps of about 2 $\mu$eV in $\varepsilon$ and possibly gate noise may reduce the flip probability compared to the Landau-Zener result. Independent measurements show that the probability for the electrons' state to change from $S$ to $T_+$ is on the order of 1/2. The quantitative details of the electronic and nuclear spin flip probabilities are currently not well understood.

[1] Foletti, S., Bluhm, H., Mahalu, D., Umansky, V. & Yacoby, A. Universal quantum control in two-electron spin quantum bits using dynamic nuclear polarization. *Nature Physics* **5**, 903 (2009).
